# Supplementary material for: Bayesian inference of ocean diffusivity from Lagrangian trajectory data
Source: arXiv:1812.04264 source file (2018-12-11)
Supplement: Supplementary file 1 [file BayesDiff_appendix_parameterisation.tex]

\section{Parameterisation of fields} \label{sec:parameterisation_fields}
In this section the parameterisation for fields used in the inference in this report are elaborated. Only linear SDEs are considered in this report. The parameterisation for the linear velocity field and the constant diffusivity tensor are thus considered in section \ref{sec:parameterisation_fields_velocity} and \ref{sec:parameterisation_fields_diffusivity}, and are summarised in \ref{sec:parameterisation_fields_linearSDE}. \par

\subsection{Linear velocity field} \label{sec:parameterisation_fields_velocity}
A linear velocity field $\vecfield{u}{x} = (u(\colvec{x}), v(\colvec{x}))^\top$ in the Cartesian coordinates $\colvec{x} = (x, y)^\top$ is given by
\begin{equation}
    \vecfield{u}{x} = \tensor{A} \left( \colvec{x} -  \colvec{x_0} \right) + \colvec{u_0}
\end{equation}
in which the matrix $\tensor{A} = \nabla \vecfield{u}{x} = \begin{bmatrix} 
            \partx{u}{x} & \partx{u}{y}   \\
            \partx{v}{x} & \partx{v}{y}  \\
        \end{bmatrix} $
represents the constant shears in the velocity field and $\colvec{u_0} = (u_0, v_0)^\top$ captures the velocity at $\colvec{x} = \colvec{x_0}$. The divergence of velocity field $\colvec{u(\colvec{x})}$ is given by the trace of matrix $\tensor{A}$, denoted as $\Tr{\tensor{A}} $, as
$$ \Tr{\tensor{A}} \equiv \partx{u}{x} + \partx{v}{y} = \nabla \cdot \colvec{u}. $$ 
An incompressible linear velocity field $\colvec{u(\colvec{x})}$ thus satisfies the zero trace condition $\Tr{\tensor{A}} = 0$.\par
To parameterise the linear velocity field, the constant component $\colvec{u_0}$ can firstly be expressed using a magnitude-angle representation, that is, 
\begin{equation} \label{eqt:u0_decomp}
    \colvec{u_0} =  \begin{pmatrix}
                        U_{0} \cos \phi_0 \\
                        U_{0} \sin \phi_0 \\
                    \end{pmatrix},
\end{equation}
in which $U_{0} = \sqrt{u_0^2 + v_0^2} \ge 0$ and $\tan \phi_0 = v_0/u_0$. \par
Secondly, the matrix $\tensor{A}$ is split into the traceless and traceful parts:
\begin{equation}
    \tensor{A} = (\tensor{A} -a\tensor{I}) + a\tensor{I},
\end{equation}
where $\tensor{I}$ is the identity matrix and $a = \frac{1}{2}\Tr{\tensor{A}}$ is half of the trace of matrix $\tensor{A}$. The traceless matrix $\tensor{A} -a\tensor{I}$ can be further decomposed into
\begin{align*}
    \tensor{A} -a\tensor{I} & = \begin{bmatrix} 
            \cos \phi_{\tensor{A}} & -\sin \phi_{\tensor{A}}   \\
            \sin \phi_{\tensor{A}} & \cos \phi_{\tensor{A}}  \\
        \end{bmatrix}
        \begin{bmatrix}
            0 & \nu_1   \\
            -\nu_2 & 0   \\
        \end{bmatrix}
        \begin{bmatrix}
            \cos \phi_{\tensor{A}}  & -\sin \phi_{\tensor{A}}   \\
            \sin \phi_{\tensor{A}}  & \cos \phi_{\tensor{A}}   \\
        \end{bmatrix}^{\top} \\
        & =
        \begin{bmatrix} 
            -\frac{1}{2}(\nu_1 - \nu_2)\sin 2\phi_{\tensor{A}} & \frac{1}{2}(\nu_1 - \nu_2)\cos 2\phi_{\tensor{A}} + \frac{1}{2}(\nu_1 + \nu_2)   \\
            \frac{1}{2}(\nu_1 - \nu_2)\cos 2\phi_{\tensor{A}} - \frac{1}{2}(\nu_1 + \nu_2) & \frac{1}{2}(\nu_1 - \nu_2)\sin 2\phi_{\tensor{A}}  \\
        \end{bmatrix},
\end{align*}
for some $\nu_1, \nu_2, \phi_{\tensor{A}} \in \mathbb{R}$ satisfying the system of equations
\begin{align*}
    \nu_1 + \nu_2 &= \partx{u}{y} - \partx{v}{x} = -\nabla \times \colvec{u}, \\
    (\nu_1 - \nu_2)\cos 2\phi_{\tensor{A}} &= \partx{u}{y} + \partx{v}{x}. \\
    (\nu_1 - \nu_2)\sin 2\phi_{\tensor{A}} &= \partx{v}{y} - \partx{u}{x}.
\end{align*}
Note that if the range of $\phi_{\tensor{A}}$ is restricted to be in $(-\pi/2, \pi/2]$ and and assuming $\nu_1 \ge \nu_2$, all three variables $\nu_1, \nu_2$ and $\phi_{\tensor{A}}$ are uniquely determined. It can furthermore be shown that $\nu_1$ and $\nu_2$ are in fact the singular values of the traceless matrix $\tensor{A} -a\tensor{I}$. \par
Note that $\nu_1$ and $\nu_2$ defined here is different from the parameterisation used in section \ref{sec:cos_shear_flow}.
Combining the traceful and traceless parts, any $2 \times 2$ real matrix $\tensor{A}$ can be expressed in the form of
\begin{equation} \label{eqt:A_decomp}
    \tensor{A} = \frac{1}{2}(\nu_1 - \nu_2) \begin{bmatrix} 
            -\sin 2\phi_{\tensor{A}} & \cos 2\phi_{\tensor{A}}   \\
            \cos 2\phi_{\tensor{A}} & \sin 2\phi_{\tensor{A}}  \\
        \end{bmatrix} 
        + 
        \frac{1}{2}(\nu_1 + \nu_2) \begin{bmatrix} 
            0 &  1   \\
            -1 & 0  \\
        \end{bmatrix} 
        + a \tensor{I}.
\end{equation} \par
As a final remark, under the representation \eqref{eqt:A_decomp}, the determinant of $\tensor{A}$ is given by $\det(\tensor{A})= a^2 + \nu_1 \nu_2$ and the eigenvalues of matrix $\tensor{A}$ are given by $a \pm \sqrt{-\nu_1 \nu_2}$. These quantities are independent of $\phi_{\tensor{A}}$ and are thus invariant to linear-affine transformation of coordinates $\colvec{x}$. \par


\subsection{Constant diffusivity field} \label{sec:parameterisation_fields_diffusivity}
A constant diffusivity field $\tensor{K}(\colvec{x})$ is represented by a symmetric positive-definite matrix $ \tensor{K} = \begin{bmatrix}
            \tensor{K}_{xx} & \tensor{K}_{xy}   \\
            \tensor{K}_{yx} & \tensor{K}_{yy}  \\
        \end{bmatrix}, $
with only $3$ degree of freedom in its representation. \par
A handy choice of parameters is motivated by the eigen-decomposition of the diffusivity tensor $\tensor{K}$:
\begin{subequations} \label{eqt:eigendecomposition_diffusivity_field}
\begin{align}
    \tensor{K}  &= 
        \begin{bmatrix} 
            \cos \phi_{\tensor{K}} & -\sin \phi_{\tensor{K}}   \\
            \sin \phi_{\tensor{K}} & \cos \phi_{\tensor{K}}  \\
        \end{bmatrix}
        \begin{bmatrix}
            {\sigma_1}^2 & 0   \\
            0 & {\sigma_2}^2  \\
        \end{bmatrix}
        \begin{bmatrix}
            \cos \phi_{\tensor{K}}  & -\sin \phi_{\tensor{K}}   \\
            \sin \phi_{\tensor{K}}  & \cos \phi_{\tensor{K}}   \\
        \end{bmatrix}^{\top}  \label{eqt:kappa_parameterisation} \\
        & =
        \begin{bmatrix}
                {\sigma_1}^2 \cos^2\phi_{\tensor{K}} + {\sigma_2}^2 \sin^2\phi_{\tensor{K}} & \left({\sigma_1}^2 - {\sigma_2}^2 \right) \cos\phi_{\tensor{K}} \sin\phi_{\tensor{K}}    \\
                \left({\sigma_1}^2 - {\sigma_2}^2 \right) \cos\phi_{\tensor{K}} \sin\phi_{\tensor{K}} & {\sigma_1}^2 \sin^2\phi_{\tensor{K}} + {\sigma_2}^2 \cos^2\phi_{\tensor{K}} \\
        \end{bmatrix},
\end{align}
\end{subequations}
where ${\sigma_1}^2, {\sigma_2}^2$ are positive real numbers and $\phi_{\tensor{K}} \in \mathbb{R}$ satisfying
\begin{align*}
    {\sigma_1}^2 + {\sigma_2}^2 &= \tensor{K}_{xx} + \tensor{K}_{yy} = \Tr{(\tensor{K})}, \\
    \left({\sigma_1}^2 - {\sigma_2}^2 \right) \cos 2\phi_{\tensor{K}}  &= \tensor{K}_{xx}  - \tensor{K}_{yy}, \\
    \left({\sigma_1}^2 - {\sigma_2}^2 \right) \sin 2\phi_{\tensor{K}} &= 2\tensor{K}_{xy}.
\end{align*}
Note that if the range of $\phi_{\tensor{K}}$ is restricted to be in $(-\pi/2, \pi/2]$ and assuming ${\sigma_1}^2 \ge {\sigma_2}^2$, all three variables ${\sigma_1}^2, {\sigma_2}^2$ and $\phi_{\tensor{K}}$ are uniquely determined for a given diffusivity tensor $\tensor{K}$.
\par
The ellipse corresponding to the quadratic equation $\colvec{x}^{\top}\tensor{K}^{-1}\colvec{x} = C$, with some constant $C$ on the $(x, y)$-plane is known as the `diffusivity ellipse'. Geometrically, $\sigma_1, \sigma_2$ are the two radii of the ellipse and $\phi_{\tensor{K}}$ is the angle between $x$-axis and the diameter with length $\sigma_1$. \par
To characterise the magnitude of diffusivity, the geometric mean $K$ of the eigenvalues of $\tensor{K}$:
\begin{equation}
    K = \sqrt{\sigma_1^2 \sigma_2^2},
\end{equation}
which coincides with the root of determinant of $\tensor{K}$ is visualised in figure \ref{fig:QGM2_DStemp_DiffusivityEllipses_diffSIv_Idx16_LocLinINC} to illustrate the spatial variation of the inferred diffusivity fields.
% It is noted from the parameterisation that the diffusivity tensor $\tensor{K}$ is periodic in $\phi_{\tensor{K}}$ with period $\pi$. In addition, that the sets of parameters $(\sigma_1, \sigma_2, \phi_{\tensor{K}}) = (a, b, \varphi)$ and $(b, a,\varphi+\frac{\pi}{2})$ result in the same diffusivity tensor $\tensor{K}$. Such periodicity and symmetry imply that the joint-distribution of $(\sigma_1, \sigma_2, \phi_{\tensor{K}})$ is necessarily multi-modal on the domain of $(\sigma_1, \sigma_2, \phi_{\tensor{K}}) \in \left( {\mathbb{R}^{+}} \right)^{2} \times \mathbb{R} $. Despite this, when the joint-distribution of $(\sigma_1, \sigma_2, \phi_{\tensor{K}})$ is mapped through \eqref{eqt:eigendecomposition_diffusivity_field} to the joint-distribution of $(\tensor{K}_{xx}, \tensor{K}_{yy}, \tensor{K}_{xy})$, the associated multi-modality in $(\sigma_1, \sigma_2, \phi_{\tensor{K}})$ collapsed into a single mode in $(\tensor{K}_{xx}, \tensor{K}_{yy}, \tensor{K}_{xy})$. Hence it is often more straightforward to interpret the joint-distribution of $(\tensor{K}_{xx}, \tensor{K}_{yy}, \tensor{K}_{xy})$ than  $(\sigma_1, \sigma_2, \phi_{\tensor{K}})$. \par 
\par

\subsection{Linear Stochastic Differential Equations} \label{sec:parameterisation_fields_linearSDE}
In \eqref{eqt:u0_decomp} and \eqref{eqt:A_decomp} it is shown that $6$ real parameters are needed to represent any linear velocity field. In \eqref{eqt:kappa_parameterisation} it is shown that $3$ real parameters are needed to parameterise a diffusivity tensor. Hence in total $9$ real variables are needed to parameterise a linear stochastic differential equation. \par
Denote $\theta_{(i)}$ as the $i$-th component of a 9-component parameter $\rowvec{\theta} = (\theta_{(1)}, \theta_{(2)}, \dots \theta_{(9)})$. Each $\theta_{(i)}$ is assigned by
\begin{subequations}
    \begin{align}
        \text{for } \colvec{u_0}:& \quad  \theta_{(1)} = U_{0}, \, \theta_{(2)} = \phi_0, \\
        \text{for } \tensor{A}:& \quad  \theta_{(3)} = \frac{1}{2} \left( \nu_1 + \nu_2 \right), \, \theta_{(4)} = \frac{1}{2} \left( \nu_1 - \nu_2 \right), \, \theta_{(5)} = 2 \phi_{\tensor{A}}, \, \theta_{(6)} = a, \\
        \text{for } \tensor{\tensor{K}}:& \quad  \theta_{(7)} = {\sigma_1}^2 - {\sigma_2}^2, \, \theta_{(8)} = {\sigma_2}^2, \, \theta_{(9)} = 2 \phi_{\tensor{K}}.
\end{align}
\end{subequations}
The posterior,a joint-distribution for the multivariate random variable $\rowvec{\theta}$, is formulated in the Bayesian methodology. Sampling algorithm can be used to analyse the $9$-dimensional probability distribution. 
\par
In addition, to enforce the incompressible condition on the inferred velocity field, it is sufficient to consider the joint-distribution of $\rowvec{\theta}$ at $\theta_{(6)}= a =\frac{1}{2}\Tr{\tensor{A}} = 0$. Similarly, for an isotropic diffusivity it suffices to consider the joint-distribution with respect to $ \theta_{(7)} = {\sigma_1}^2 - {\sigma_2}^2 = 0$ and $\theta_{(9)} = 2 \phi_{\tensor{K}} = 0$. If altogether the no shear is inferred, studying the distribution with vanishing $\theta_{(3)}, \theta_{(4)}, \theta_{(5)}$ and $\theta_{(6)}$ will provide the inference. \par
